# Supplementary material for: Multi-Agent Safe Planning with Gaussian Processes
Source: arXiv:2008.04452 source file (2020-08-10)
Supplement: Supplementary file 1 [file appendix.tex]

\subsection{Code Submission}
The code can be found in the folder named ``multiagent-safemdp". To execute the code, you need to have Python 3.7, Scikit-learn, Pytorch and Anaconda installed. Please run:\\
%\begin{lstlisting}
\texttt{conda install gdal}\\
%\end{lstlisting}
so that the package for downloading mars map. 

There are two experiments in our paper. 

The code for Mars rover experiment can be executed with the following command\\
\texttt{python main.py}\\
where the arguments are specified at the top of the main.py file.

The code for quadcopter can be executed with the following command\\
\texttt{python quadcopter/runsim.py}\\
where the arguments are prespecified in the experiment.

\subsection{Proofs}
\textbf{Theorem 5.1.}
\textit{If $\beta^i_r(t)$ is chosen as $\beta^i_r(t) = 2B + 300\alpha_t\log^3(t/\delta)$, agent $i$'s historical states all visited by the estimating agent and $Q$ is in the form of universal representation of states, with at least probability $1 - \delta^i$, $Q(s, a) \in C_{Q_t}(s, a)$, where $\delta^i$ is the agent $i$'s probability of visiting unsafe states.}
\begin{proof}
\cite{turchetta2016safe} proved that with the choice of $\beta^i_r(t)$ above, there is at least probability $1 - \delta^i$, $r(s^i) \in {C_{r_t}}(s^i), \forall s^i \in \mathcal{S}$. The Q-learning algorithm we define is by sampling potential transitions (to $s'$) and perform
\begin{equation}
Q_t(s^i, a^i) = r_t(s') + \gamma \max_{a'}Q_t(s', a')
\end{equation}
Hence at convergence with a universal representation of Q-function, the Q-function can be defined as
\begin{equation}
Q_t(s^i, a^i) =   \mathbb{E}[r_t(s')] + \gamma \mathbb{E}[r_t(s'')] + \gamma^2 \mathbb{E}[r_t(s''')] + \dots
\end{equation}
where we use $s'$, $s''$, $s'''$, $\dots$ denote the future states distributions in the optimal trajectory of taking $a^i$ at $s^i$, and this holds for each of $Q_t^\mu, Q_t^l$, and $Q_t^u$ respectively with $r_t^\mu, r_t^l$, and $r_t^u$. Since $\forall s \in S$, $r_t(s) \in C_{r_t}(s)$ with probability at least $1-\delta^i$. Hence $\mathbb{E}[r_t(s')] \in [\mathbb{E}[r_t^l(s')], \mathbb{E}[r_t^u(s')]]$, with probability at least $1-\delta^i$ for any state distribution. Therefore with probability at least $1-\delta^i$,
\begin{equation}\label{value_func_var}
\begin{split}
    Q_t(s^i, a^i) \in &[\mathbb{E}[r_t^l(s')] + \gamma\mathbb{E}[r_t^l(s'')] + \gamma^2\mathbb{E}[r_t^l(s''')] + \dots,\\ 
    & \mathbb{E}[r_t^u(s')] + \gamma\mathbb{E}[r_t^u(s'')] + \gamma^2\mathbb{E}[r_t^u(s''')] + \dots]\\
    & = [Q^l_t(s^i, a^i), Q^u_t(s^i, a^i)] \qedhere
\end{split}
\end{equation}
\end{proof} 

\textbf{Theorem 5.2.}
\textit{$Q^u_t(s, a) - Q^l_t(s, a) \leq \frac{2\beta_r(t)\max_{s \in S} \sigma_{r_t}(s)}{1-\gamma}$ for discounted infinite time horizon MDP, $\forall s, a \in \mathcal{S}, \mathcal{A}$ and any given $\beta_r(t)$ as a constant for $C_{r_t}(s)$. }

\begin{proof}
	As stated in the proof above, at convergence with a universal representation of Q-function, the Q-function can be defined as
	\begin{equation}
	Q_t(s^i, a^i) =   \mathbb{E}[r_t(s')] + \gamma \mathbb{E}[r_t(s'')] + \gamma^2 \mathbb{E}[r_t(s''')] + \dots
	\end{equation}
	where we use $s'$, $s''$, $s'''$, $\dots$ denote the next state distribution in the optimal trajectory of taking $a^i$ at $s^i$, and this holds for each of $Q_t^\mu, Q_t^l$, and $Q_t^u$ respectively with $r_t^\mu, r_t^l$, and $r_t^u$. Hence,	
	\begin{equation}\label{value_func_var2}
	\begin{split}
	&Q^u_t(s, a) - Q^l_t(s, a) \\
	& =( \mathbb{E}[r^u(s')] + \gamma \mathbb{E}[r^u(s'')] + \gamma^2 \mathbb{E}[r^u(s''')] + \dots ) - ( \mathbb{E}[r^l(s')] + \gamma \mathbb{E}[r^l(s'')] + \gamma^2 \mathbb{E}[r^l(s''')] + \dots)\\
	& = ( \mathbb{E}[r^u(s') - r^l(s')] + \gamma \mathbb{E}[r^u(s'') - r^l(s'')] + \gamma^2 \mathbb{E}[r^u(s''') - r^l(s''')] + \dots ),\\
	&\text{by linearity of expectation}\\
	& \leq 2\beta_r(t) \mathbb{E}[\sigma_{r_t}(s')]) + 2\gamma\beta_r(t) \mathbb{E}[\sigma_{r_t}(s'')] + 2\gamma^2\beta_r(t) \mathbb{E}[\sigma_{r_t}(s''')]) + \dots \\
	%& \text{variance of correlated Gaussian variables' sum is less than the sum of the variances of the variables}\\
	& = 2\beta_r(t) (\mathbb{E}[\sigma_{r_t}(s')] + \gamma \mathbb{E}[\sigma_{r_t}(s'')] +  \gamma^2 \mathbb{E}[\sigma_{r_t}(s''')]) + \dots\\
	& \leq \frac{2\beta_r(t)\max_s \sigma_{r_t}(s)}{1-\gamma}\text{, since $\mathbb{E}[\sigma_{r_t}(s')] \leq max_{s\in S} \sigma_{r_t}(s) \text{ } \forall s'$ as a distribution of states in $S$} \qedhere
	\end{split}
	\end{equation}
\end{proof} 

\textbf{Theorem 5.3.}
\textit{The Multi-agent SafeMDP algorithm has a time complexity of $O(|\mathcal{S}|^3 + Nt)$ at time step $t$ in a MA-MDP with $N$ agents.}

\begin{proof}
	With the prior knowledge that Gaussian Process updates are $O(|\mathcal{S}|^3)$ \cite{rasmussen2004gaussian}, we can derive the time complexity bounds as follows.
	
	There are four major components of this algorithm.
	Gaussian Process update for the reward function is on the state space and for all agents, hence complexity $O(|\mathcal{S}|^3)$. Q-function update with sampling takes $O(1)$. Optimization for $\epsilon$ and $T^i_b$ is linear to the number of steps in trajectory, hence complexity $O(Nt)$.
	
	Incorporating all complexity bounds above, the time complexity bound of the algorithm is $O(|\mathcal{S}|^3 + Nt)$. \qedhere
\end{proof}
